# Supplementary material for: New Algorithms for Minimizing the Weighted Number of Tardy Jobs On a Single Machine
Source: arXiv:1709.05751 source file (2017-09-18)
Supplement: Supplementary file 1 [file appendix.tex]

\textbf{\label{A1}The proof of Lemma~\ref{lol}:}

Consider first the set of constraints in (\ref{set3}) when $i$ is fixed. Due
to the sorting rule in (\ref{weight_sort}), we have that
\begin{equation}
(y_{i}-j+1)w_{ij}+\sum_{l=1}^{j-1}w_{il}\leq
(y_{i}-j)w_{i,j+1}+\sum_{l=1}^{j}w_{il}  \label{h1}
\end{equation}%
when $1\leq j\leq y_{i}$; and that
\begin{equation}
(y_{i}-j+1)w_{ij}+\sum_{l=1}^{j-1}w_{il}\geq
(y_{i}-j)w_{i,j+1}+\sum_{l=1}^{j}w_{il}  \label{h2}
\end{equation}%
when $y_{i}+1\leq j\leq n_{i}-1$. The fact that (\ref{h1})\ and (\ref{h2})
holds leads to the conclusion that the maximal value of the term in the
right side of (\ref{set3}) is when either $j=y_{i}$ or $j=y_{i}+1$. However,
the fact that the value of this term is identical for both cases when either
$j=y_{i}$ or $j=y_{i}+1$, and is equal to $\sum_{l=1}^{y_{i}}w_{il}$, leads
to the conclusion that the tightest constraints among the $n_{i}$
constraints in set (\ref{set3}) are those related to $j=y_{i}$ and $%
j=y_{i}+1 $, while all other are redundant. Accordingly, for any feasible $%
y_{i}$ value, set (\ref{set3}) is equivalent to
\begin{equation*}
z_{i}\geq \sum_{l=1}^{y_{i}}w_{il}\text{.}
\end{equation*}%
The fact that our objective is to minimize $Z_{T}$ in (\ref{obj}) further
implies that in an optimal solution the relation in (\ref{relation})\ holds.

\paragraph{\label{A2}The proof of Lemma~\ref{lol2}}
The fact that $y^{\prime }=y^{\ast }$ implies that the objective value in (%
\ref{obj2}) is identical for both $S^{\prime }$ and $S^{\ast }$. Thus, in
order to prove that $S^{\prime }$ is optimal to \emph{P3.1 }it remains to
prove that it satisfy the constraints in (\ref{const1.1}),(\ref{const1.2})
and (\ref{const1.3}). By the definition of $x^{\prime }$ above we have that $%
x_{ij}^{\prime }\leq m_{ij}$ for $i\in \{1,...,k\}$ and $j\in \{1,...,l\}$.
Therefore $x^{\prime }$ satisfy the set of conditions in (\ref{const1.1}).
The fact that $S^{\ast }$ is feasible solution implies that $%
\sum_{i=1}^{k}\sum_{r=1}^{j}p_{i}x_{ir}^{\ast }\leq d_{j}$ for $j=1,...,l$.
(see (\ref{const1.3})). The fact that $S^{\ast }$ is feasible solution
implies that $n_{i}-\sum_{j=1}^{l}x_{ij}^{\ast }=y_{i}^{\ast }$ for $%
i=1,...,k$ (see (\ref{const1.2})). Since $x_{i}^{\prime
}=\sum_{j=1}^{l}x_{ij}^{\prime }=\sum_{j=1}^{r_{i}-1}x_{ij}^{\prime
}+x_{ir_{i}}^{\prime }+\sum_{j=r_{i}+1}^{l}x_{ij}^{\prime }=0+(x_{i}^{\ast
}-\sum_{j=r_{i}+1}^{l}m_{ij})+\sum_{j=r_{i}+1}^{l}m_{ij}=x_{i}^{\ast
}=\sum_{j=1}^{l}x_{ij}^{\ast }$ and $y^{\prime }=y^{\ast }$ this further
implies that $n_{i}-\sum_{j=1}^{l}x_{ij}^{\prime }=y_{i}^{\prime }$ for $%
i=1,...,k$ and therefore $S^{\prime }$ satisfy the set of conditions in (\ref%
{const1.2}) as well. By definition of $x^{\prime }$, setting $x=x^{\prime }$
minimizes the value of $\sum_{r=1}^{j}x_{ir}$ for $j=1,...,l$, subject to
the restriction that $\sum_{j=1}^{l}x_{ij}=x_{i}^{\ast }$. Therefore we have
that $\sum_{i=1}^{k}\sum_{r=1}^{j}p_{i}x_{ir}^{\prime }\leq
\sum_{i=1}^{k}\sum_{r=1}^{j}p_{i}x_{ir}^{\ast }\leq d_{j}$, and $S^{\prime }$
satisfy the set of conditions in (\ref{const1.3}) as well. Thus, $S^{\prime }
$ is an optimal solution for \emph{P3.1.}

The fact that all $x_{ij}^{\prime }$ values are integer, implies that $%
S^{\prime }$ is feasible (and therefore also optimal)\ for \emph{P3 }as well.

\paragraph{\label{A3}The proof of Lemma~\ref{L5}}
First note that the two partial schedules has the same partial objective
value of $\Sigma_{i=1}^{w_{\#}} w_{i}(n_{ij}-e_{i})$, where $n_{ij}$ be the
number of jobs of type $i$ in job set $\{J_{1},...,J_{j}\}$. Now, consider a
feasible extension of $S_{2}$ to a complete schedule. The fact that $%
P_{E}(S_{1})\leq P_{E}(S_{2})$ implies that the same extension is feasible
for partial schedule $S_{1}$ as well. Therefore, for any complete schedule
which is an extension of $S_{2}$, we can construct a complete schedule with
the same objective value out of $S_{1}$. This completes our proof.

\paragraph{\label{A4}The proof of Lemma~\ref{L6}}
First note that in both partial schedules the total processing time of the
early sets is identical, i,e., $P_{E}(S_{1})=P_{E}(S_{2})=\Sigma
_{i=1}^{p_{\#}}p_{i}e_{i}$. Now, consider a feasible extension of $S_{2}$ to
a complete schedule. The fact that $P_{E}(S_{1})=P_{E}(S_{2})$ implies that
the same extension is feasible for partial schedule $S_{1}$ as well, and the
theorem follows.

\end{document}
